# Supplementary material for: The Expected Number of Roots over The Field of p-adic Numbers
Source: arXiv:2101.03561 source file (2021-11-21)
Supplement: Supplementary file 1 [file appendix_a.tex]

\section{Roots of random integral polynomials}
\label{app:rationals-roots}

Consider the random polynomial 
\[
f\pa*{X}=\rC_{0}+\rC_{1}X+\dots+\rC_{n-1}X^{n-1}+X^{n}
\]
where $\rC_{0},\dots,\rC_{n-1}$ are i.i.d. random variables distributed
according to a law $\mu$ -- a probability measure on the ring $R$. We denote
by $\rCount f$ the number of roots of $f$ without multiplicities i.e.
\[
\rCount f=\#\set*{ r\in R:f\pa*{r}=0} \text{.}
\]
We prove a theorem presented in the thesis which
says that for $R=\ZZ$, the value of $\Ex\br*{\rCount f}$
converges to $\Pr\pa*{\rC_{0}=0}$ as $n\to\infty$. Formally,
\begin{thm}
\label{thm:rational-root-count}
Let $f\pa*{X}=\rC_{0}+\rC_{1}X+\dots+\rC_{n-1}X^{n-1}+X^{n}$
be a random polynomial where $\rC_{0},\dots,\rC_{n-1}$ are i.i.d.
non-constant random variables taking values in $\ZZ$.
Assume that there exists $\varepsilon>0$
such that $\Ex\br*{\abs*{\rC_{i}}^{\varepsilon}}<\infty$.
Then
\[
\Ex\br*{\rCount f}=\Pr\pa*{\xi_{0}=0}+O\pa*{n^{-3/10}}
\]
as $n\to\infty$.
\end{thm}

\begin{lem}
\label{lem:rational-root-prob}
\[
\Pr\pa*{f\text{ has a root}\cond\rC_{0}\ne0}=O\pa*{n^{-3/10}}
\]
as $n\to\infty$.
\end{lem}

\begin{proof}
This follows from \cite[Proposition 2.1]{bary-soroker_irreducibility_2020}.
Denote by $H$ the event $\abs*{\rC_{i}}\le\exp\pa*{n^{1/3}}$
for all $i=0,\dots,n-1$ and by $R_{t}$ the event that $f$ has an
irreducible factor of degree $\le t$. In particular, $R_{1}$ is the
event that $f$ has a root. By the law of total probability
\begin{align}
\Pr\pa*{R_{1}\cond\rC_{0}\ne0} & =\Pr\pa*{R_{1}\cond\rC_{0}\ne0,H}\Pr\pa*{H}+\Pr\pa*{R_{1}\cond\rC_{0}\ne0,H^{\comp}}\Pr\pa*{H^{\comp}}\label{eq:r1-prob-bound}\\
 & \le\Pr\pa*{R_{1}\cond\rC_{0}\ne0,H}+\Pr\pa*{H^{\comp}}\text{.}\nonumber 
\end{align}

To bound $\Pr\pa*{R_{1}\cond\rC_{0}\ne0,H}$, let $\mu_n$ be the
probability measure defined by
$$ \mu_n\pa*{E} = \frac{\mu\pa*{E\cap B_n}}{\mu\pa*{B_n}}, $$
where $B_n = \br*{-\exp\pa*{n^{1/3}}, \exp\pa*{n^{1/3}}} \cap \ZZ$.
Note that $\mu_n$ is the common law of $\rC_{0},\dots,\rC_{n-1}$ conditioned
on $H$. From the continuity of measures we have that $\mu\pa*{B_n}\xrightarrow{n\to\infty} 1$.
Hence, $\left\lVert \mu_n\right\rVert_{\infty}\xrightarrow{n\to\infty} \left\lVert \mu\right\rVert_{\infty}$. Since the variables $\rC_{0},\dots,\rC_{n-1}$ are non-constant, we have
that $\left\lVert \mu\right\rVert _{\infty}<1$.
So, for $n$ sufficiently large
we have that
$$\left\lVert \mu_n\right\rVert_{\infty} <1-n^{-1/10}.$$
%We apply \cite[Proposition 2.1]{bary-soroker_irreducibility_2020} to get that
We now have the requirements to apply \cite[Proposition 2.1]{bary-soroker_irreducibility_2020}:
\begin{equation}
\Pr\pa*{R_{1}\cond\rC_{0}\ne0,H}\le
\Pr\pa*{R_{n^{-1/10}}\cond\rC_{0}\ne0,H}=O\pa*{n^{-3/10}}
\text{.}\label{eq:r1-cond-prob-bound}
\end{equation}

Next, we bound $\Pr\pa*{H^{\comp}}$. We have 
\begin{align}
\Pr\pa*{H^{\comp}} & =1-\Pr\pa*{H}\label{eq:not-bounded-prop}\\
 & =1-\Pr\pa*{\forall i,\abs*{\rC_{i}}\le\exp\pa*{n^{1/3}}}\nonumber \\
 & =1-\Pr\pa*{\abs*{\rC_{0}}\le\exp\pa*{n^{1/3}}}^{n}\nonumber \\
 & =1-\pa*{1-\Pr\pa*{\abs*{\rC_{0}}>\exp\pa*{n^{1/3}}}}^{n}\text{.}\nonumber 
\end{align}
By Markov inequality we have
\[
\Pr\pa*{\abs*{\rC_{0}}>\exp\pa*{n^{1/3}}}=\Pr\pa*{\abs*{\rC_{0}}^{\varepsilon}>\exp\pa*{\varepsilon n^{1/3}}}\le\Ex\br*{\abs*{\rC_{0}}^{\varepsilon}}\exp\pa*{-\varepsilon n^{1/3}}\text{.}
\]

Plugging this into (\ref{eq:not-bounded-prop}) gives
\begin{align}
\Pr\pa*{H^{\comp}} & \le1-\pa*{1-\Ex\br*{\abs*{\rC_{0}}^{\varepsilon}}\exp\pa*{-\varepsilon n^{1/3}}}^{n}\label{eq:hc-prob-bound}\\
 & =1-\pa*{1+O\pa*{n\exp\pa*{-\varepsilon n^{1/3}}}}\nonumber \\
 & =O\pa*{n\exp\pa*{-\varepsilon n^{1/3}}}\text{.}\nonumber 
\end{align}

We finish the proof by plugging equations (\ref{eq:r1-cond-prob-bound})
and (\ref{eq:hc-prob-bound}) in equation (\ref{eq:r1-prob-bound}).
\end{proof}
\begin{lem}
\label{lem:non-zero-rational-root-prob}
\[
\Pr\pa*{f\text{ has a non-zero root}}=O\pa*{n^{-3/10}}
\]
as $n\to\infty$.
\end{lem}

\begin{proof}
Denote the event that $f$ has a non-zero root by $Z_{f}$ and put
$q=\Pr\pa*{\rC_{0}=0}$. We prove by induction on $n=\deg f$
that
\begin{equation}
\Pr\pa*{Z_{f}}\le c_{1}q^{n}\sum_{k=1}^{n}k^{-3/10}q^{-k}\label{eq:z-prob-induction-bound}
\end{equation}
for some constant $c_{1}>0$ which is independent of $n$.

First, we find the constant $c_{1}$. By Lemma~\ref{lem:rational-root-prob},
there exists a constant $c_{2}>0$ such that
\[
\Pr\pa*{f\text{ has a root}\cond\rC_{0}\ne0}\le c_{2}n^{-3/10}
\]
 for all positive integers $n$. We put $$c_{1}=\pa*{1-q}\max\pa*{1,c_{2}}.$$

For the basis of induction, we have that $f=X-\rC_{0}$. Hence,
\[
\Pr\pa*{Z_{f}}=\Pr\pa*{\rC_{0}\ne0}=1-q\le c_{1}\text{.}
\]
For the induction step, we assume that equation~\eqref{eq:z-prob-induction-bound}
holds for a random polynomial of degree $n-1$ distributed as above. By the law of total probability
\begin{equation}
\Pr\pa*{Z_{f}}=\Pr\pa*{Z_{f}\cond\rC_{0}\ne0}\Pr\pa*{\rC_{0}\ne0}+\Pr\pa*{Z_{f}\cond\rC_{0}=0}\Pr\pa*{\rC_{0}=0}\text{.}\label{eq:z-prob-total-prob}
\end{equation}
When $\rC_{0}\ne0$, the event $Z_f$ occurs if and only if $f$ has
a root. So
\begin{equation}
\Pr\pa*{Z_{f}\cond\rC_{0}\ne0}=\Pr\pa*{f\text{ has a root}\cond\rC_{0}\ne0}\le c_{2}n^{-3/10}\text{.}\label{eq:z-prob-non-zero-free-coeff}
\end{equation}
If $\rC_{0}=0$, then $X^{-1}f\pa*{X}$ has the same non-zero
roots as $f$. Moreover,
\[
X^{-1}f\pa*{X}=\rC_{1}+\rC_{2}X+\dots+X^{n-1}\text{.}
\]
Hence by the induction hypothesis, we get that
\begin{equation}
\Pr\pa*{Z_{f}\cond\rC_{0}=0}=\Pr\pa*{Z_{X^{-1}f\pa*{X}}\cond\rC_{0}=0}\le c_{1}q^{n-1}\sum_{k=1}^{n-1}k^{-3/10}q^{-k}\text{.}\label{eq:z-prob-induction-used}
\end{equation}
We plug equations \eqref{eq:z-prob-non-zero-free-coeff} and (\ref{eq:z-prob-induction-used})
into equation \eqref{eq:z-prob-total-prob} to get
\begin{align*}
\Pr\pa*{Z_{f}} & \le c_{2}n^{-3/10}\pa*{1-q}+\pa*{c_{1}q^{n-1}\sum_{k=1}^{n-1}k^{-3/10}q^{-k}}q\\
 & \le c_{1}n^{-3/10}+c_{1}q^{n}\sum_{k=1}^{n-1}k^{-3/10}q^{-k}\\
 & \le c_{1}q^{n}\sum_{k=1}^{n}k^{-3/10}q^{-k}\text{,}
\end{align*}
as needed for the induction.

Next, we bound the growth rate of the sum $\sum_{k=1}^{n}k^{-3/10}q^{-k}$.
We split the sum into two smaller sums:
\begin{equation}\label{eq:series-split}
  \sum_{k=1}^{n}k^{-3/10}q^{-k} =
    \sum_{k=1}^{\left\lceil n/2\right\rceil-1} k^{-3/10}q^{-k}
    + \sum_{k=\left\lceil n/2\right\rceil}^{n} k^{-3/10}q^{-k}
\end{equation}
We bound the first sum trivially:
\[
  \sum_{k=1}^{\left\lceil n/2\right\rceil-1} k^{-3/10}q^{-k}
  \le \sum_{k=1}^{\left\lceil n/2\right\rceil-1} q^{-n/2}
  \le \frac{n}{2} q^{-n/2}
  \text{.}
\]
For the second sum, we use the geometric series:
\[
  \sum_{k=\left\lceil n/2\right\rceil}^{n} k^{-3/10}q^{-k}
  \le \sum_{k=\left\lceil n/2\right\rceil}^{n} {\pa*{\frac{n}{2}}}^{-3/10}q^{-k}
  = {\pa*{\frac{n}{2}}}^{-3/10} O\pa*{q^{-n}}
  \text{.}
\]

Returning to equation \eqref{eq:series-split} we get
\[
\sum_{k=1}^{n}k^{-3/10}q^{-k}
  = O\pa*{nq^{-n/2} + n^{-3/10} q^{-n}} = O\pa*{n^{-3/10} q^{-n}}
\]
Therefore,
$$
q^n \sum_{k=1}^{n}k^{-3/10}q^{-k}
  = O\pa*{n^{-3/10}}
\text{,}
$$
which finishes the proof applying equation~\eqref{eq:z-prob-induction-bound}.
\end{proof}
\begin{proof}[Proof of Theorem~\ref{thm:rational-root-count}]
Denote by $\rCountX f$ the number of non-zero rationals roots of $f$.
Obviously, we have $\rCount f=\ind{f\pa*{0}=0}+\rCountX f$.
Let
$$d\pa*{n}=\#\set*{d > 0 : d\mid n}$$
be
the divisor function.
For any $\varepsilon > 0$ there exists $c_1>0$ such that
$d\pa*{n} \le c_1 n^\varepsilon$, see \cite[page 296]{apostol_introduction_1998}.
We let $K =  \max\pa*{2, c_{1}\Ex\br*{\abs*{\rC_{0}}^{\varepsilon}\cond\rCountX f\ne0,\rC_{0}\ne0}}$. Then we note that
\begin{equation}
\Ex\br*{d\pa*{\rC_{0}}\cond\rCountX f\ne0,\rC_{0}\ne0}
\le K
\text{.}\label{eq:c1-inequality}
\end{equation}

We prove by induction on $n$ that 
\begin{equation}
\Ex\br*{\rCountX f\cond\rCountX f\ne0}\le K-q^{n}\label{eq:non-zero-root-count-bound}
\end{equation}
where $q=\Pr\pa*{\rC_{i}=0}$.

For $n=1$, equation~\eqref{eq:non-zero-root-count-bound}
follows immediately since $\rCountX f\le1$. Next we assume equation~\eqref{eq:non-zero-root-count-bound} 
holds true for a random polynomial of degree $n-1$ distributed as above.
Then by the law of total expectation
\begin{multline*}
\Ex\br*{\rCountX f\cond\rCountX f\ne0}=\Ex\br*{\rCountX f\cond\rCountX f\ne0,\rC_{0}=0}\Pr\pa*{\rC_{0}=0}\\
+\Ex\br*{\rCountX f\cond\rCountX f\ne0,\rC_{0}\ne0}\Pr\pa*{\rC_{0}\ne0}\text{.}
\end{multline*}
When $\rC_{0}\ne0$, by the rational root theorem all the roots of $f$
must divide $\rC_{0}$. Hence $\rCountX f\le d\pa*{\rC_{0}}$
and by equation (\ref{eq:non-zero-root-count-bound}) we have 
\[
\Ex\br*{\rCountX f\cond\rCountX f\ne0,\rC_{0}\ne0}\le K\text{.}
\]
If $\rC_{0}=0$ then the polynomial $X^{-1}f\pa*{X}$ has the
same non-zero roots as $f$. Also,
\[
X^{-1}f\pa*{X}=\rC_{1}+\rC_{2}X+\dots+\rC_{n-2}X^{n-2}+X^{n-1}\text{.}
\]
Thus, we can use the induction hypothesis to infer that 
\[
\Ex\br*{\rCountX f\cond\rCountX f\ne0,\rC_{0}=0}=\Ex\br*{\rCountX{\frac{f\pa*{X}}{X}}\cond\rCountX f\ne0,\rC_{0}=0}\le K-q^{n-1}\text{.}
\]
Therefore 
\[
\Ex\br*{\rCountX f\cond\rCountX f\ne0}\le\pa*{K-q^{n-1}}q+K\pa*{1-q}=K-q^{n}\text{,}
\]
and equation~\eqref{eq:c1-inequality} is proved.

To finish the proof, we use again the law of total expectation to
get
\[
\Ex\br*{\rCountX f}=\Ex\br*{\rCountX f\cond\rCountX f\ne0}\Pr\pa*{\rCountX f\ne0}\text{.}
\]
By equation (\ref{eq:non-zero-root-count-bound}) we get that
\[
\Ex\br*{\rCountX f}\le\pa*{K-q^{n}}\Pr\pa*{\rCountX f\ne0}\le K\Pr\pa*{\rCountX f\ne0}
\text{,}
\]
which can be written as
\[
\Ex\br*{\rCountX f}=\Pr\pa*{\rCountX f\ne0}O\pa*{1}\text{.}
\]
Applying Lemma~\ref{lem:non-zero-rational-root-prob} we get that $\Pr\pa*{\rCountX f\ne0}=O\pa*{n^{-3/10}}$
hence finishing the proof.
\end{proof}
